# Supplementary material for: Time Series Continuous Modeling for Imputation and Forecasting with Implicit Neural Representations
Source: arXiv:2306.05880 source file (2024-04-22)
Supplement: Supplementary file 1 [file figure_INR_explain.tex]

\begin{figure*}[!htb]
    \centering
    \includegraphics[width=0.70\linewidth]{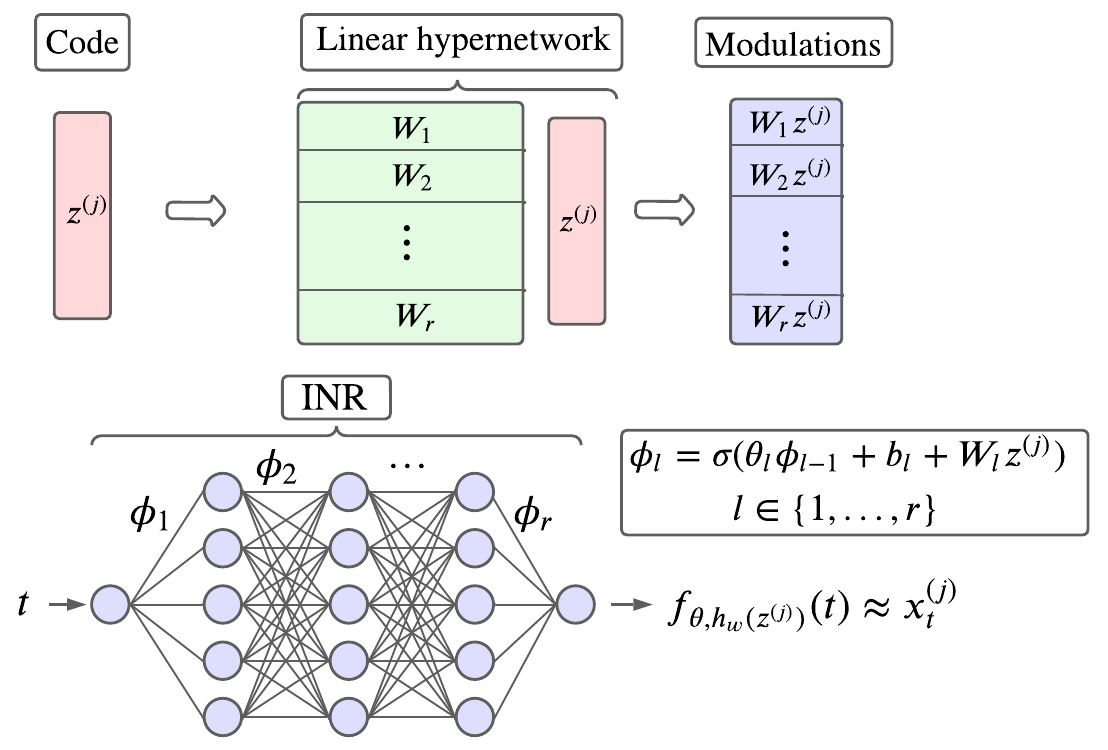}
    \caption{Architecture overview. $\sigma$ stands for a point-wise activation function}
    \label{fig:inr_explain}
\end{figure*}
