# Supplementary material for: Time Series Continuous Modeling for Imputation and Forecasting with Implicit Neural Representations
Source: arXiv:2306.05880 source file (2024-04-22)
Supplement: Supplementary file 2 [file figures_joint_varying_lbw_h.tex]

\begin{figure*}[t!]
    \centering
    \begin{subfigure}[t]{0.5\textwidth}
        \includegraphics[width=0.99\linewidth]{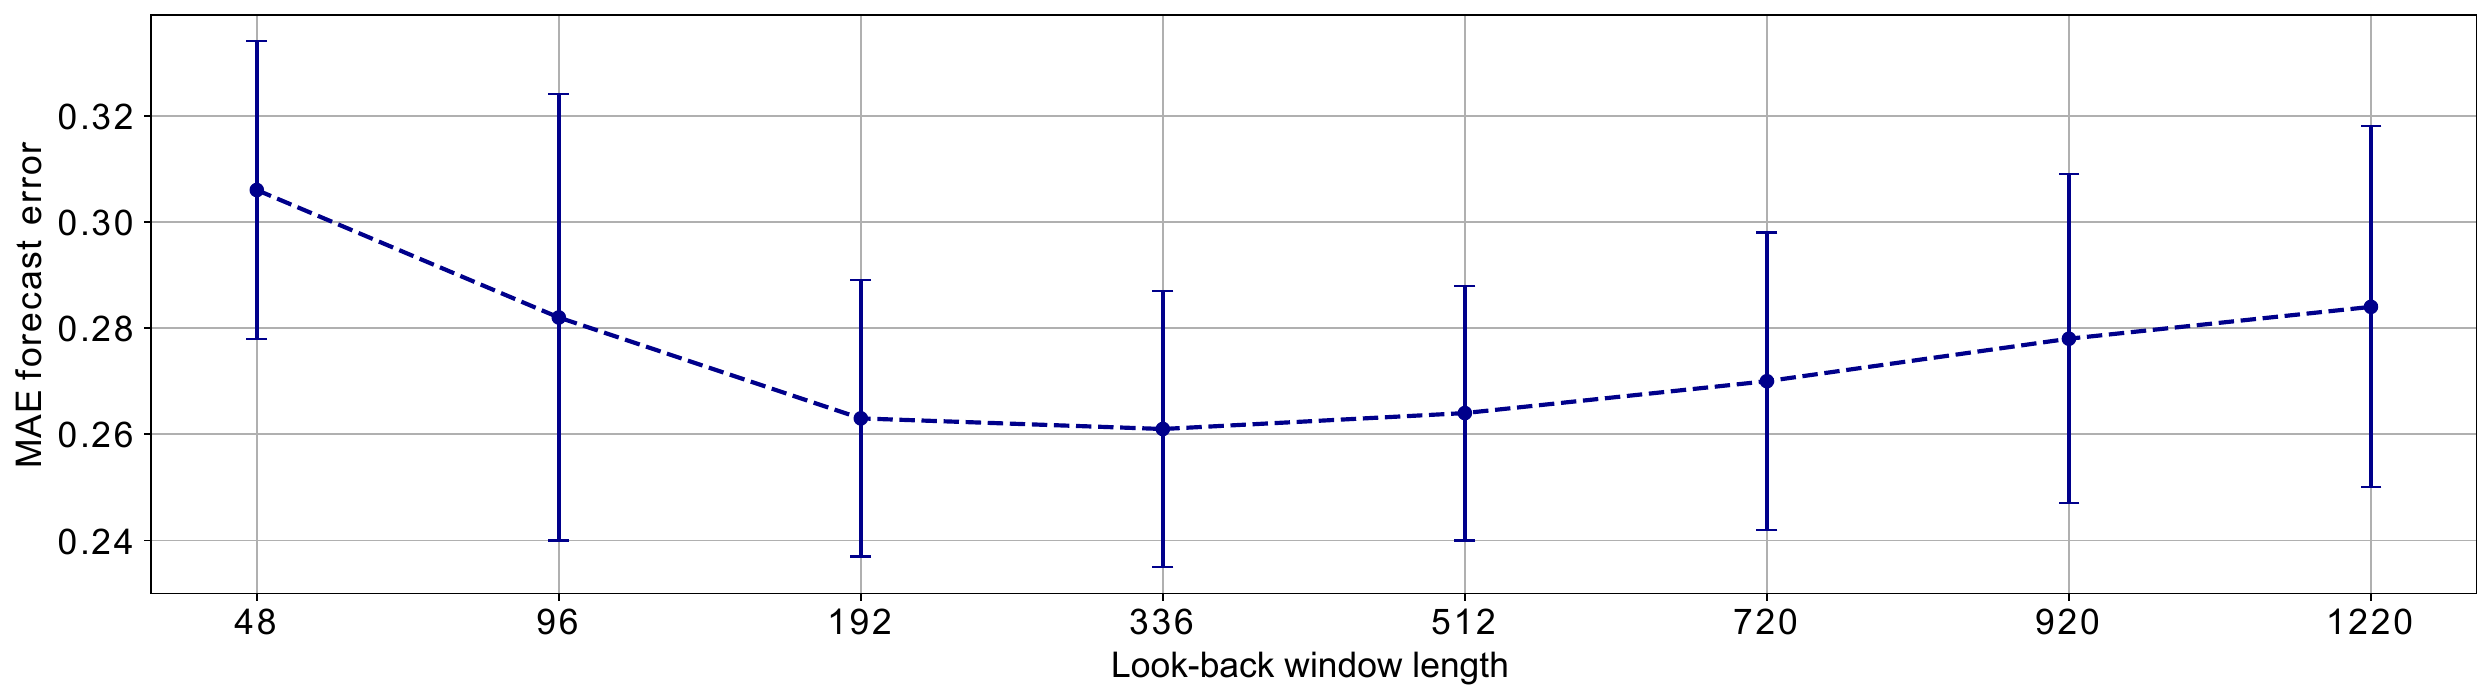}
        \caption{MAE error per look-back windows for the \textit{Electricity} dataset (horizon window is 336 length). Models are trained on a given time window and test on 4 time window.}
    \end{subfigure}%
    ~ 
    \begin{subfigure}[t]{0.5\textwidth}
        \centering
        \includegraphics[width=0.99\linewidth]{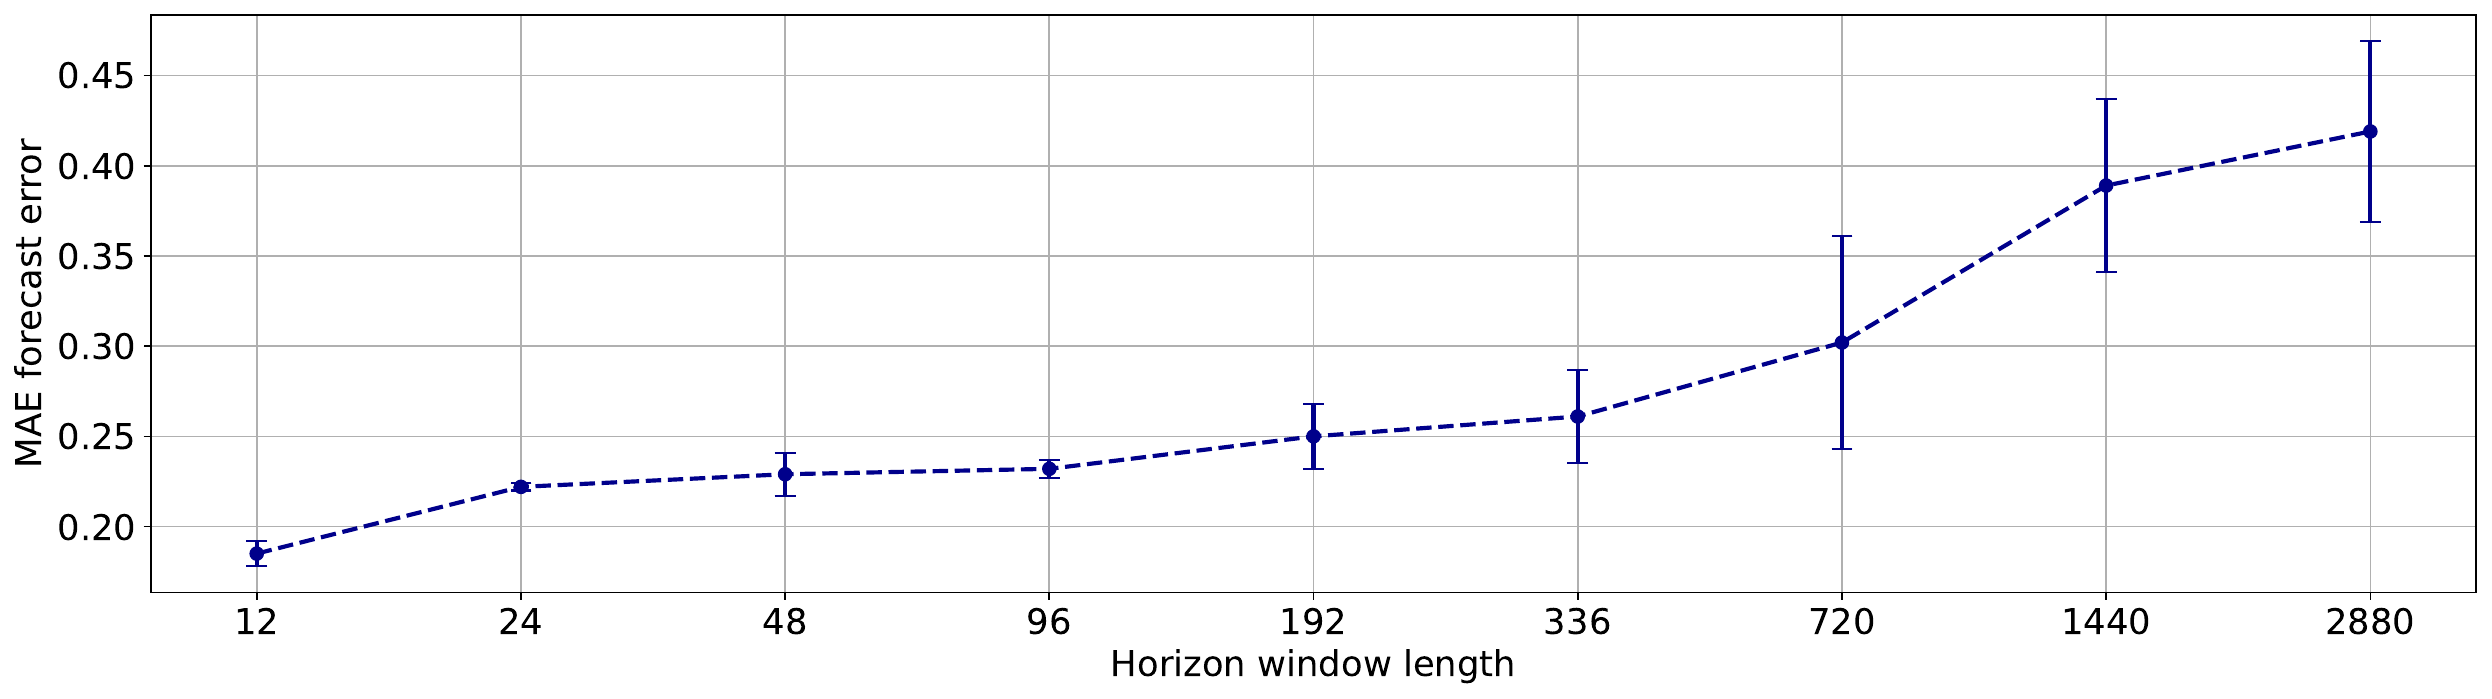}
        \caption{MAE error per horizons for the \textit{Electricity} dataset (look-back window is 512). Models are trained on a given time window and test on 4 time window.}
    \end{subfigure}
    \caption{Caption place holder}
\end{figure*}
