# Supplementary material for: Time Series Continuous Modeling for Imputation and Forecasting with Implicit Neural Representations
Source: arXiv:2306.05880 source file (2024-04-22)
Supplement: Supplementary file 4 [file table_transfer_electricity.tex]

\begin{table}[!t]

\setlength{\tabcolsep}{5pt}
\caption{MAE results for Electricity forecasting. Transfer table.}
\label{tab:transfer_elec}
\begin{center}
\scalebox{0.75}{%
\begin{tabular}{cccccc}
\toprule[1.5pt]
  & H  &     TimeFlow & PatchTST & DeepTime \\                          
  
        \midrule
         \multirow{2}{*}{Electricity $\to$ Electricity} & 96 & 0.228 $\pm$ 0.028 & 0.221 $\pm$ 0.023 & 0.244 $\pm$ 0.026\\
         &  192  & 0.238 $\pm$ 0.020 & 0.229 $\pm$ 0.020 & 0.252 $\pm$ 0.019\\
                                     
        \midrule
         \multirow{2}{*}{Traffic $\to$ Electricity} & 96 & 0.277 $\pm$ 0.03 & 0.257 $\pm$ 0.018 & 0.255 $\pm$ 0.023\\
         &  192  & 0.286 $\pm$ 0.019  & 0.264 $\pm$ 0.016 & 0.256 $\pm$ 0.014\\

         \midrule

         \multirow{2}{*}{SolarH $\to$ Electricity} & 96 & 0.526 $\pm$ 0.029 & 0.327 $\pm$ 0.028 & 0.292 $\pm$  0.022 \\
         &  192  & 0.529 $\pm$ 0.037 & 0.334 $\pm$ 0.028 & 0.301 $\pm$ 0.025 \\
        
        \bottomrule[1.5pt]

\end{tabular}}
\end{center}
\end{table}
