# Supplementary material for: Time Series Continuous Modeling for Imputation and Forecasting with Implicit Neural Representations
Source: arXiv:2306.05880 source file (2024-04-22)
Supplement: Supplementary file 5 [file figure_setting_imputation_procedure.tex]

\begin{figure*}[!htb]
    \centering
    \includegraphics[width=0.99\linewidth]{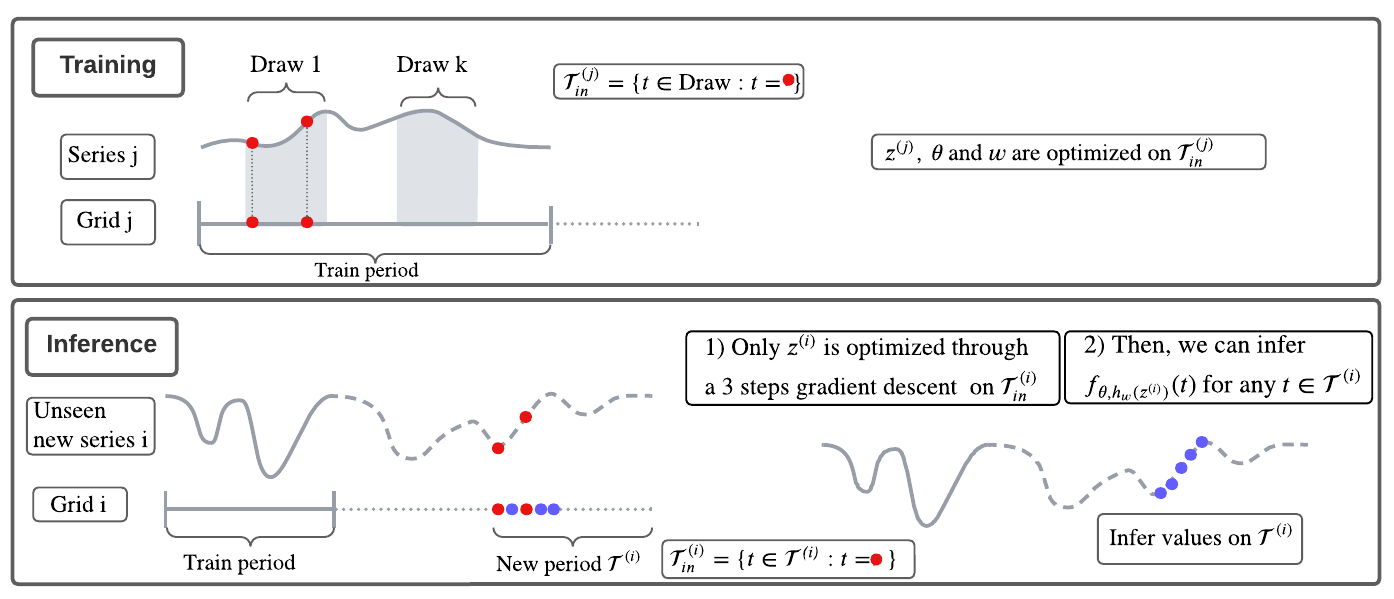}
    \caption{Training and inference procedures for imputation for new samples on new periods}
    \label{fig:imputation_procedure_new_samples}
\end{figure*}
