# Supplementary material for: Time Series Continuous Modeling for Imputation and Forecasting with Implicit Neural Representations
Source: arXiv:2306.05880 source file (2024-04-22)
Supplement: Supplementary file 6 [file mTan_training_plot.tex]

\begin{figure}[H]
    \centering
    \includegraphics[width=0.60\linewidth]{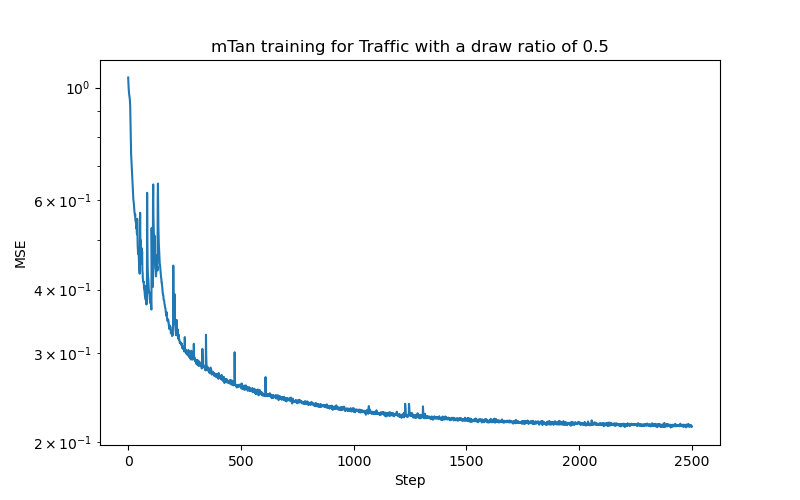}
    \caption{MAE training curve of mTan for the \textit{Traffic} dataset with a draw ratio of 0.5.}
    \label{fig:mTan_training}
\end{figure}
