# Supplementary material for: Time Series Continuous Modeling for Imputation and Forecasting with Implicit Neural Representations
Source: arXiv:2306.05880 source file (2024-04-22)
Supplement: Supplementary file 7 [file imputation_NeuralProcess.tex]

\begin{table}[H]

\setlength{\tabcolsep}{4pt}
\caption{Mean MAE imputation results on the missing grid only over five different time windows. $\tau$ stands for the subsampling rate. Bold results are best, underline results are second best.}

\label{tab:impu_classic_plus_neural_process}
\begin{center}
\scalebox{0.66}{%
\begin{tabular}{cccccccccc}
\toprule
  & $\tau$ &  TimeFlow & SAITS & BRITS & TIDER & mTAN & Linear & KNN (k=3) & Neural Process\\
\midrule

        & 0.05 &  \textbf{0.324 $\pm$ 0.013}    &   0.384 $\pm$ 0.019     & \underline{0.329 $\pm$ 0.015} & 0.427 $\pm$ 0.010 & 0.575 $\pm$ 0.039  & 0.828 $\pm$ 0.045 & 0.531 $\pm$ 0.033 & 0.417 $\pm$ 0.057 \\

        & 0.10 &  \textbf{0.250 $\pm$ 0.010}    &    0.308 $\pm$ 0.011   &  \underline{0.287 $\pm$ 0.015} & 0.399 $\pm$ 0.009 & 0.412 $\pm$ 0.047 & 0.716 $\pm$ 0.039 & 0.416 $\pm$ 0.020 & 0.357 $\pm$ 0.015\\

        Electricity & 0.20 &  \textbf{0.225 $\pm$ 0.008}    &   0.261 $\pm$ 0.008    &  \underline{0.245 $\pm$ 0.011} & 0.391 $\pm$ 0.010 & 0.342 $\pm$ 0.014 & 0.518 $\pm$ 0.029 &  0.363 $\pm$ 0.019 & 0.320 $\pm$ 0.017 \\

        & 0.30 &  \textbf{0.212 $\pm$ 0.007}    &    0.236 $\pm$ 0.008  &  \underline{0.221 $\pm$ 0.008} & 0.384 $\pm$ 0.009 &0.335 $\pm$ 0.015 & 0.396 $\pm$ 0.022 & 0.342 $\pm$ 0.017 & 0.300 $\pm$ 0.022\\

        & 0.50 &  \underline{0.194 $\pm$ 0.007}   &    0.209  $\pm$ 0.008 &  \textbf{0.193 $\pm$ 0.008} & 0.386 $\pm$ 0.009 & 0.340 $\pm$ 0.022 & 0.275 $\pm$ 0.015 &  0.323 $\pm$ 0.016 & 0.297 $\pm$ 0.016 \\ %Tider best res for 0.5 is with previous setting
        
        \midrule

        & 0.05 &  \textbf{0.095 $\pm$ 0.015}    &   0.142 $\pm$ 0.016   &  0.165 $\pm$ 0.014 & 0.291 $\pm$ 0.009  & 0.241 $\pm$ 0.102 & 0.339 $\pm$ 0.031 & 0.151 $\pm$ 0.017 & \underline{0.115 $\pm$ 0.015}\\

        & 0.10 &  \textbf{0.083 $\pm$ 0.015}    &     0.124  $\pm$ 0.018  &  0.132 $\pm$ 0.015 & 0.276 $\pm$ 0.010 & 0.251 $\pm$ 0.081 & 0.170 $\pm$ 0.014 & 0.128 $\pm$ 0.017 & \underline{0.114 $\pm$ 0.014}\\

        Solar & 0.20 &  \textbf{0.072 $\pm$ 0.015}   &     0.108  $\pm$ 0.014 &  0.109 $\pm$ 0.012 & 0.270 $\pm$ 0.010 & 0.314 $\pm$ 0.035 & \underline{0.088 $\pm$ 0.010} & 0.110 $\pm$ 0.016 & 0.109 $\pm$ 0.016 \\

        & 0.30 &   \textbf{0.061 $\pm$ 0.012}   &     0.100 $\pm$ 0.015   &  0.098 $\pm$ 0.012 & 0.266 $\pm$ 0.010 & 0.338 $\pm$ 0.05 & \underline{0.063 $\pm$ 0.009} & 0.103 $\pm$ 0.017 & 0.108 $\pm$ 0.016 \\

        & 0.50 &   \underline{0.054 $\pm$ 0.013}   &     0.094 $\pm$ 0.013   &  0.088 $\pm$ 0.013 & 0.262 $\pm$ 0.009 & 0.315 $\pm$ 0.080 & \textbf{0.044 $\pm$ 0.008} & 0.096 $\pm$ 0.016 &  0.107 $\pm$ 0.015\\

        \midrule

        & 0.05 &  \underline{0.283 $\pm$ 0.016}    &    0.293 $\pm$ 0.007   & \textbf{0.261 $\pm$ 0.010} & 0.363 $\pm$ 0.007 & 0.406 $\pm$ 0.074 & 0.813 $\pm$ 0.027 &  0.387 $\pm$ 0.014 & 0.318 $\pm$ 0.014\\

        & 0.10 &  \textbf{0.211 $\pm$ 0.012}    &    \underline{0.237 $\pm$ 0.006}   &  0.245 $\pm$ 0.009 & 0.362 $\pm$ 0.006 & 0.319 $\pm$ 0.025 & 0.701 $\pm$ 0.026 &  0.293 $\pm$ 0.012 & 0.288 $\pm$ 0.018 \\

        Traffic & 0.20 &  \textbf{0.168 $\pm$ 0.006}    &     \underline{0.197 $\pm$ 0.005}  & 0.224 $\pm$ 0.008 & 0.361 $\pm$ 0.006 & 0.270 $\pm$ 0.012 & 0.508 $\pm$ 0.022 & 0.249 $\pm$ 0.010 & 0.271 $\pm$ 0.011 \\

        & 0.30 &  \textbf{0.151 $\pm$ 0.007}    &   \underline{0.180  $\pm$ 0.006}   & 0.197 $\pm$ 0.007 &  0.355 $\pm$ 0.006 % with lr 0.005
        & 0.251 $\pm$ 0.006 & 0.387 $\pm$ 0.018 &  0.228 $\pm$ 0.009 & 0.259 $\pm$ 0.012 \\

        & 0.50 &  \textbf{0.139 $\pm$ 0.007}    &    \underline{0.160  $\pm$ 0.008}  &  0.161 $\pm$ 0.060 & 0.354 $\pm$ 0.007 & 0.278 $\pm$ 0.040 & 0.263 $\pm$ 0.013 &  0.204 $\pm$ 0.009 & 0.240 $\pm$ 0.021\\
        \bottomrule

\end{tabular}}
\end{center}
\end{table}
