# Supplementary material for: Time Series Continuous Modeling for Imputation and Forecasting with Implicit Neural Representations
Source: arXiv:2306.05880 source file (2024-04-22)
Supplement: Supplementary file 8 [file table_variation_code_dimension.tex]

\begin{table}[!h]
\caption{MAE imputation errors on the first time window of \textit{Electricity} dataset. Best results are bold.}
\label{tab:Zdimension}
\begin{center}
\scalebox{0.65}{
\begin{tabular}{cccccc}
\toprule
    & $\tau$ & $\text{dim}(z)=32$  & $\text{dim}(z)=64$ & $\text{dim}(z)=128$ & $\text{dim}(z)=256$ \\
        \midrule
        \multirow{5}{*}{Electricity} & 0.05 & 0.370 & 0.364 & \textbf{0.323} & 0.354\\

        & 0.10 & 0.302 & 0.301 & \textbf{0.252} & 0.283\\

        & 0.20 & 0.269 & 0.265 & \textbf{0.224} & 0.247 \\

        & 0.30 & 0.242 & 0.245 & \textbf{0.211} & 0.238 \\

        & 0.50 & 0.224 & 0.240 & \textbf{0.194} & 0.217 \\

        \bottomrule

\end{tabular}}
\end{center}
\end{table}
